# Supplementary material for: Controlling crackling dynamics by triggering low intensity avalanches
Source: arXiv:2010.14807 ancillary file (2020-10-28)
Supplement: Supplementary file 1 [file TriggerCleverSM.pdf]

# Supplementary materials for : Controlling crackling dynamics by triggering low intensity avalanches

Jonathan Barés, Daniel Bonamy

October 27, 2020

## 1 Complementary figures for avalanche size PDF

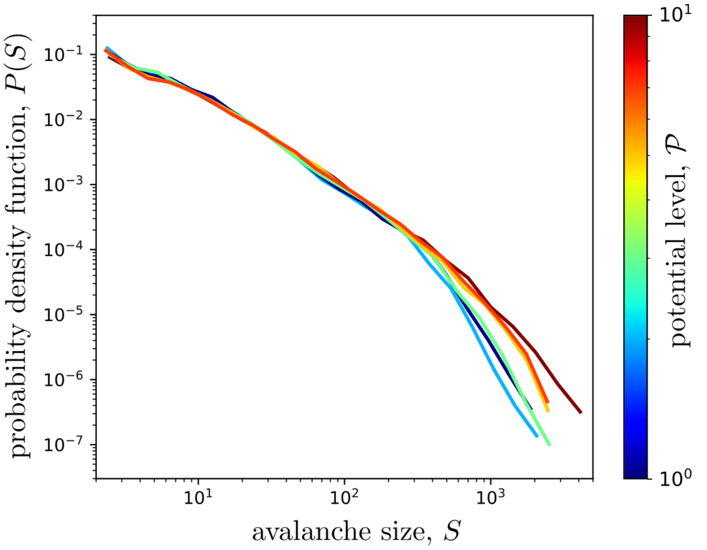


Figure 1: PDFs of the avalanche size, $P(S)$. Results are shown for simulations with random excitation, considering only the non-triggered avalanches, with $\mathcal{A} = 200$, $\mathcal{T} = 20$ and varying $\mathcal{P}$.

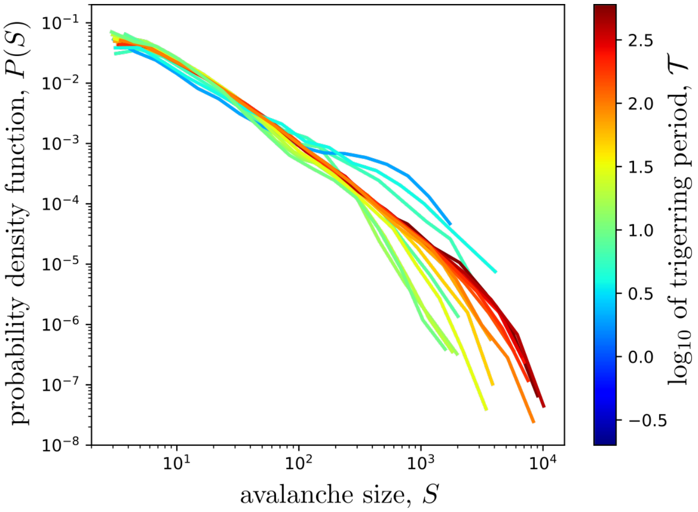


Figure 2: PDFs of the avalanche size, $P(S)$. Results are shown for simulations with random excitation, considering only the non-triggered avalanches, with $\mathcal{A} = 200$, $\mathcal{P} = 2$ and varying $\mathcal{T}$.

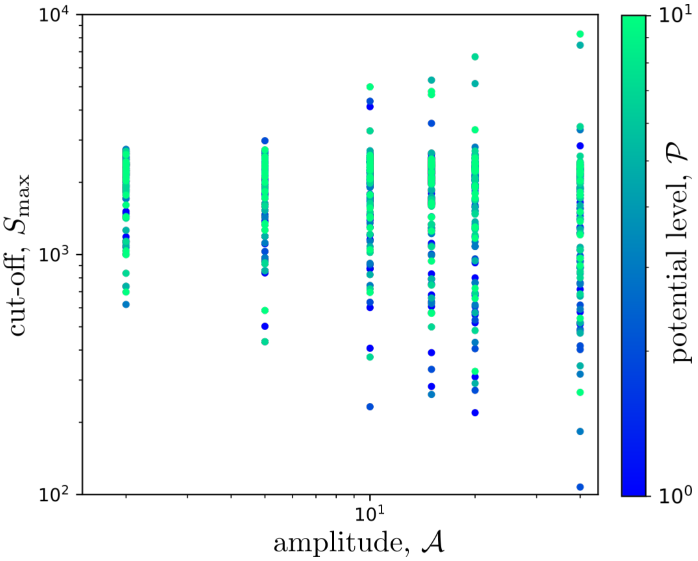


Figure 3: Evolution of the $P(S)$ upper cut-offs as a function of the excitation amplitude $\mathcal{A}$ for simulations with any $\mathcal{P}$ and $\mathcal{T}$. In these statistical analysis triggered avalanches are not considered.

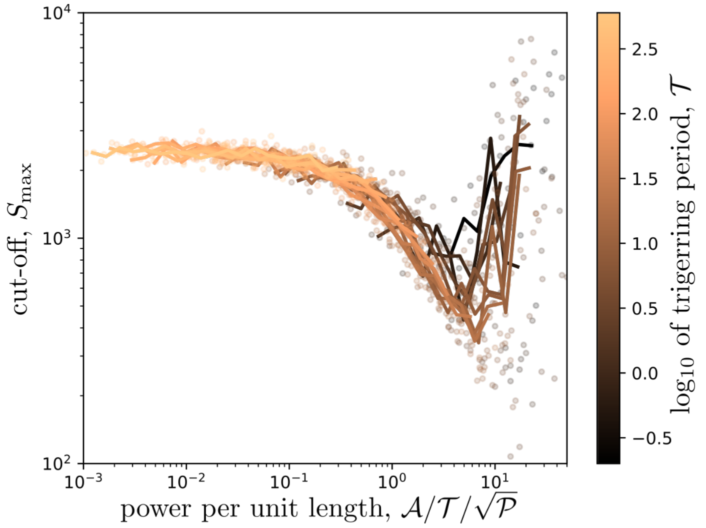


Figure 4: Evolution of the $P(S)$ upper cut-offs as a function of the power density $\mathcal{Q} = \mathcal{A}/\mathcal{T}/\sqrt{\mathcal{P}}$. Solid curves show average results for constant $\mathcal{T}$. In these statistical analysis triggered avalanches are not considered but all simulations for any $\mathcal{A}$, $\mathcal{T}$ and $\mathcal{P}$ values are considered.

## 2 Complementary figures for waiting time PDF

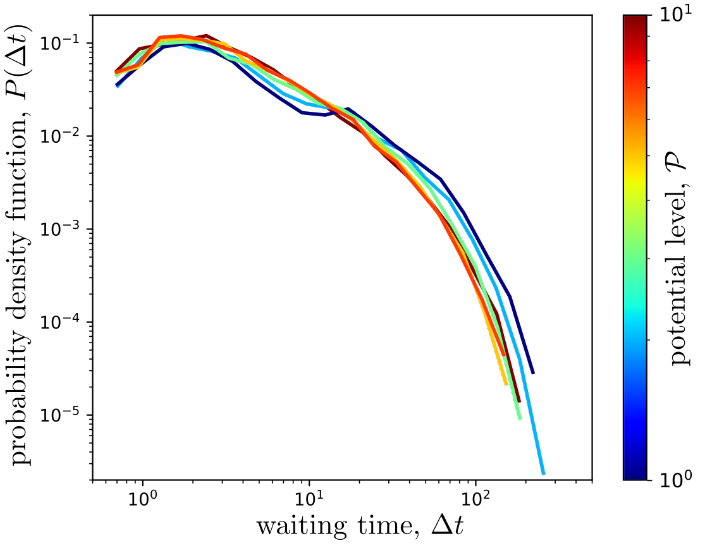


Figure 5: PDFs of the waiting time between two consecutive avalanches, $P(\Delta t)$. Results are shown for simulations with random excitation, considering only the non-triggered avalanches, with $\mathcal{A} = 200$, $\mathcal{T} = 20$ and varying $\mathcal{P}$.

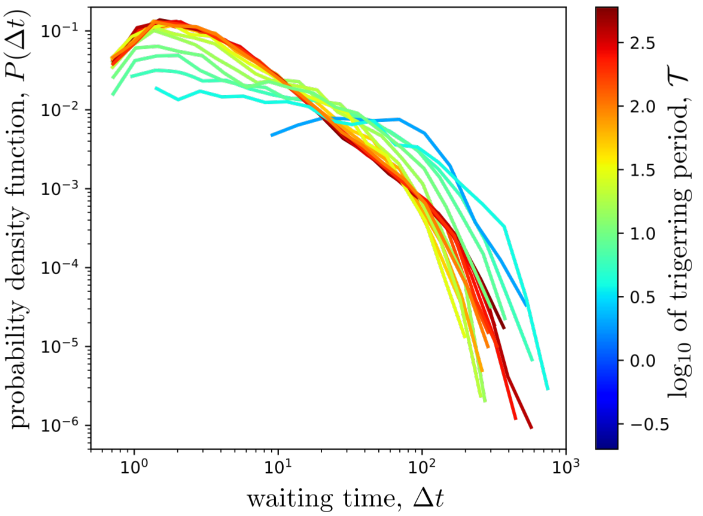


Figure 6: PDFs of the waiting time between two consecutive avalanches, $P(\Delta t)$. Results are shown for simulations with random excitation, considering only the non-triggered avalanches, with $\mathcal{A} = 200$, $\mathcal{P} = 2$ and varying $\mathcal{T}$.

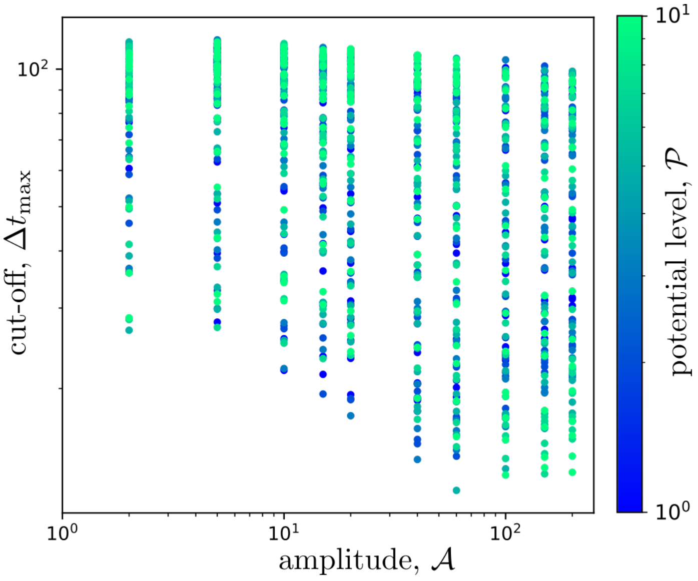


Figure 7: Evolution of the $P(\Delta t)$ upper cut-offs as a function of the excitation amplitude $\mathcal{A}$ for simulations with any $\mathcal{P}$ and $\mathcal{T}$. In these statistical analysis triggered avalanches are not considered.

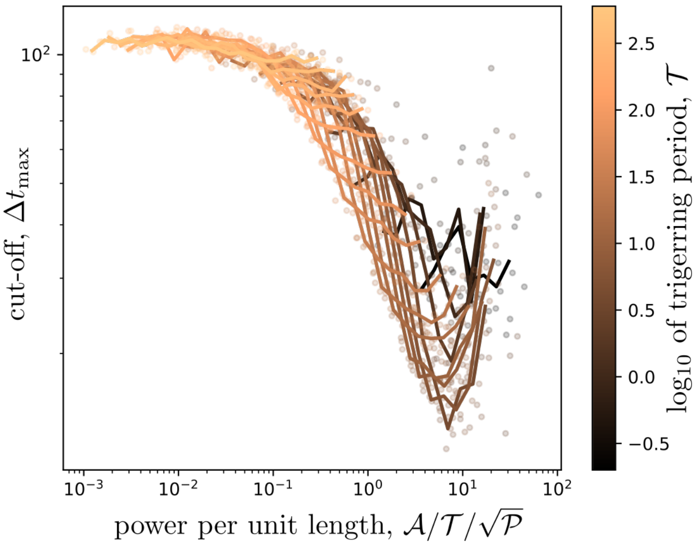


Figure 8: Evolution of the $P(\Delta t)$ upper cut-offs as a function of the power density $\mathcal{Q} = \mathcal{A}/\mathcal{T}/\sqrt{\mathcal{P}}$. Solid curves show average results for constant $\mathcal{T}$. In these statistical analysis triggered avalanches are not considered but all simulations for any $\mathcal{A}$, $\mathcal{T}$ and $\mathcal{P}$ values are considered.

## 3 Complementary figures for avalanche rate

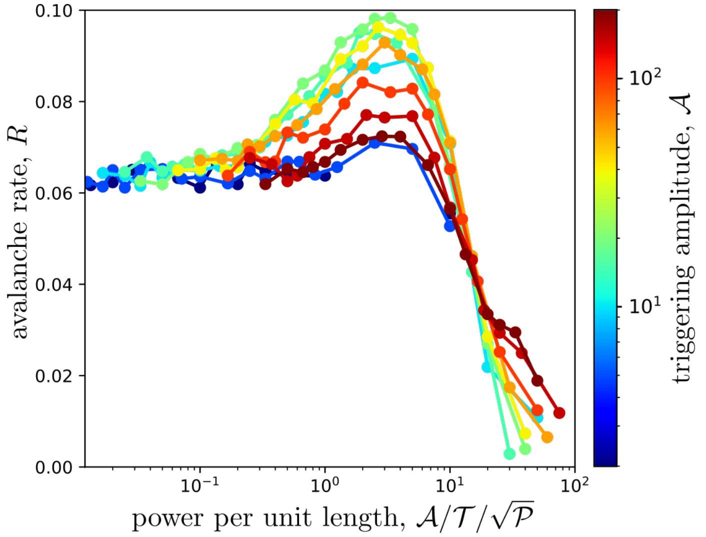


Figure 9: Number of avalanche per unit time, $R$, and avalanche shape asymmetry as a function of the power density $\mathcal{Q}$. Statistics are plotted for simulations with random excitation removing triggered avalanches. $\mathcal{P}$ is fixed to 2.

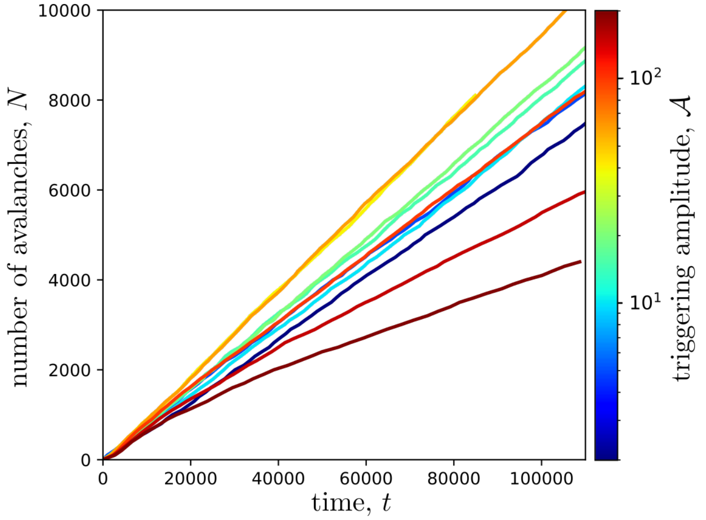


Figure 10: Evolution of the number avalanches as a function of time for simulations with random excitation without considering triggered avalanches for $\mathcal{P} = 2$ and $\mathcal{T} = 20$.

# 4 Complementary figure for avalanche shape

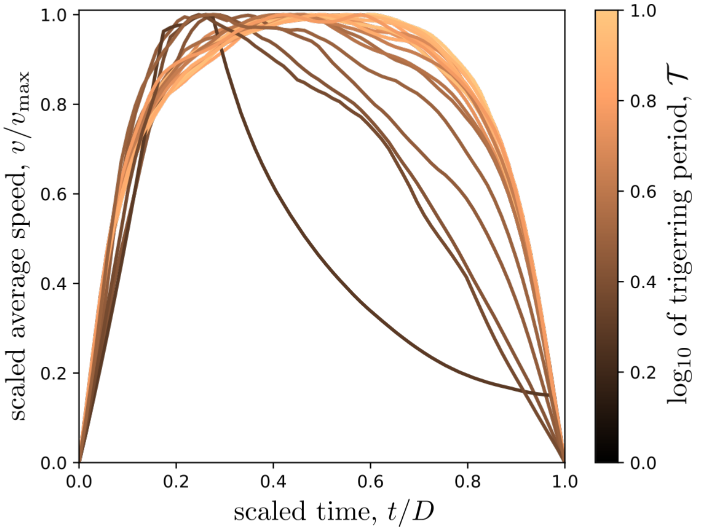


Figure 11: Avalanche shape, plotted as the scaled front speed as a function of the time scaled with the avalanche duration for avalanches with durations between 3 and 5. Results are presented for simulations with random excitation removing triggered events for $\mathcal{A} = 200$ and $\mathcal{P} = 2$

# 5 Example movie

Example of front propagation simulation with random excitations for $\mathcal{A} = 200$, $\mathcal{T} = 20$ and $\mathcal{P} = 2$. By sake of clarity the whole system is not shown but a reduced band in the middle of the random field. Clear areas that suddenly appear in ahead of the crack front are excitation burst.

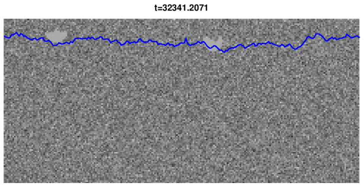


Figure 12: Snapshot of a simulation with with random excitations for $\mathcal{A} = 200$, $\mathcal{T} = 20$ and $\mathcal{P} = 2$
